# Supplementary material for: Capital growth since the 19th century
Source: arXiv:2610.38997 source file (2026-10-28)
Supplement: Supplementary file 1 [file tbl-wid_si_table.tex]

\centering
\begin{tabularx}{\columnwidth}{lcc}
   Regression of $\Delta s^*$ on $\Delta g(K)$   & 0.0202$^{***}$\\   
                                                 & (0.0075)\\   
   Observations                                  & 2,347\\  
   R$^2$                                         & 0.48557\\  
   Within R$^2$                                  & 0.04003\\  
    \\
   Year fixed effects                            & $\checkmark$\\   
   Country fixed effects                         & $\checkmark$\\   
\end{tabularx}
   \label{tbl-wid_si_table}
